# Supplementary material for: The effect of iron layer thickness on the interlayer exchange coupling in Fe/MgO (001) superlattices
Source: arXiv:2401.08336 source file (2024-04-23)

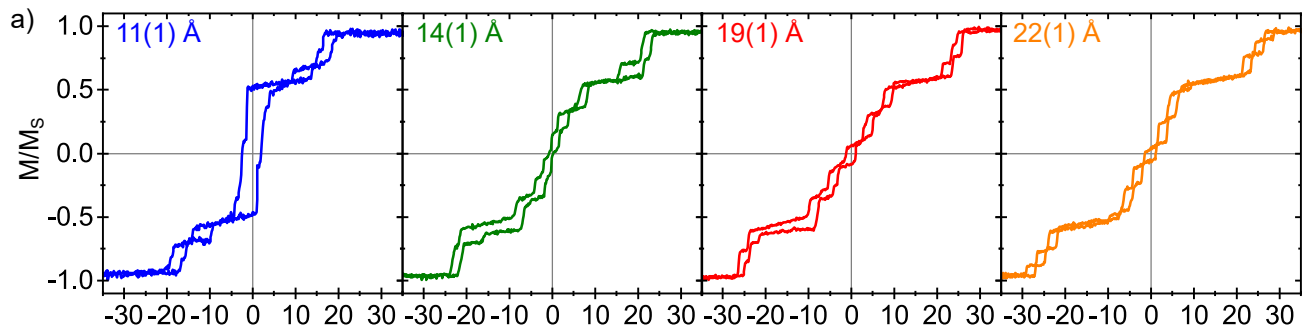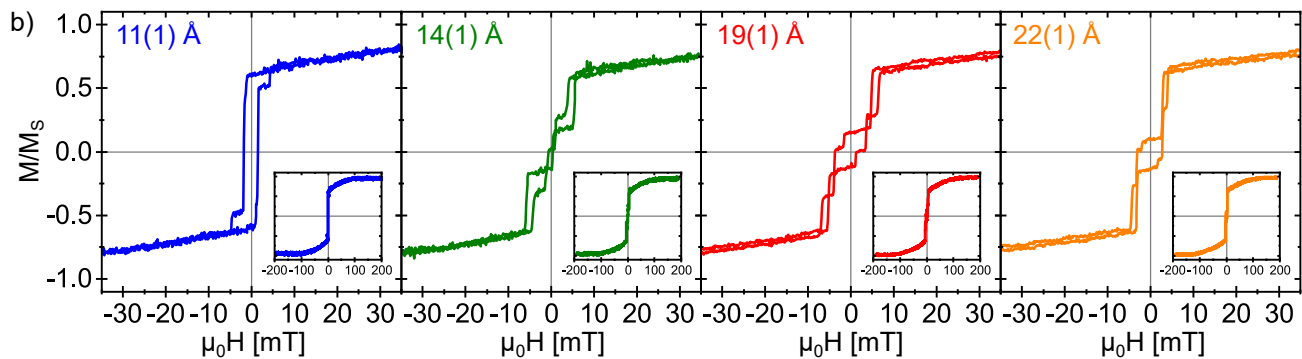

Supplement: Supplementary file 1 [file Figure1_Supp.pdf]
